# Supplementary material for: Sector models - A toolkit for teaching general relativity: III. Spacetime geodesics
Source: arXiv:1804.09765 ancillary file (2018-04-25)

Worksheets for

Sector models—A toolkit for teaching general relativity:

III. Spacetime geodesics

[www.spacetime.travel.org/sectormodels3](http://www.spacetime.travel.org/sectormodels3)

Arbeitsmaterialien zu

Sektormodelle – Ein Werkzeugkasten zur Vermittlung der Allgemeinen  
Relativitätstheorie: III. Geodäten in der Raumzeit

[www.tempolimit-lichtgeschwindigkeit.de/sectormodels3](http://www.tempolimit-lichtgeschwindigkeit.de/sectormodels3)

Ute Kraus, Corvin Zahn, Universität Hildesheim, 2018

## Minkowski diagram

The story of the lion and the gazelle

## Minkowskidiagramm

Die Geschichte vom Löwen und von der Gazelle

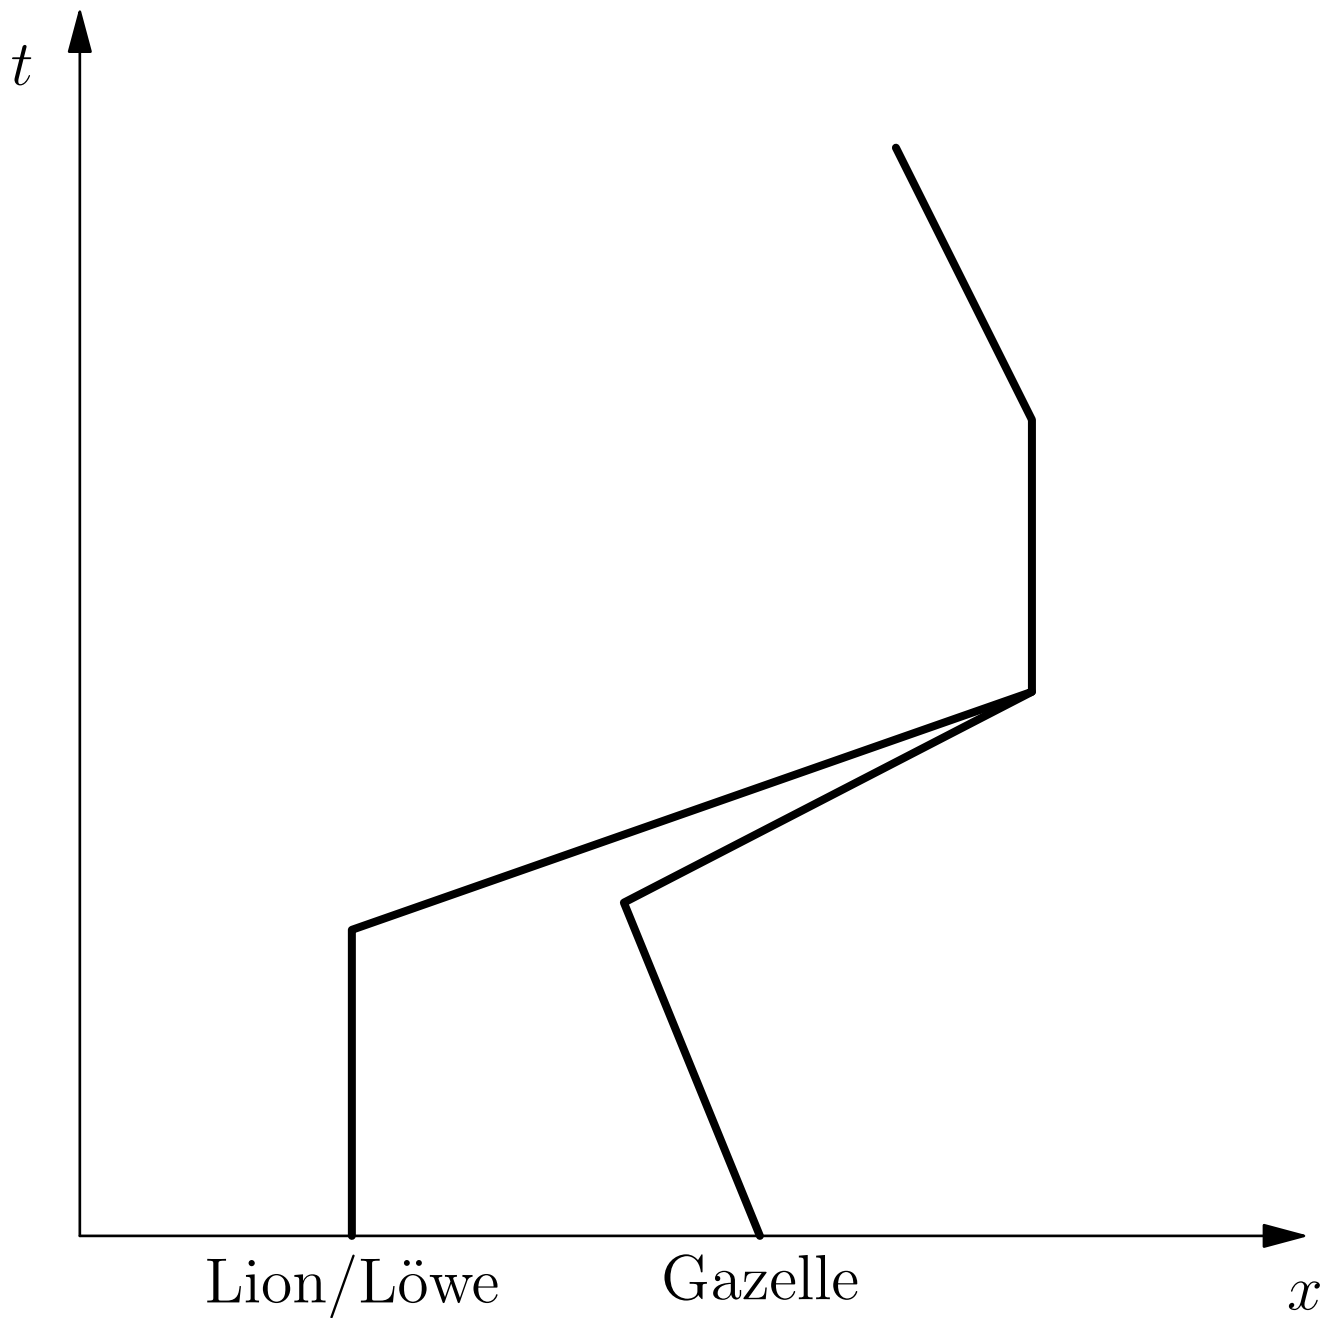

Sector model of the spacetime of a radial ray in the exterior region of a black hole

Sektormodell für die Raumzeit eines radialen Strahls im Außenraum eines Schwarzen Lochs

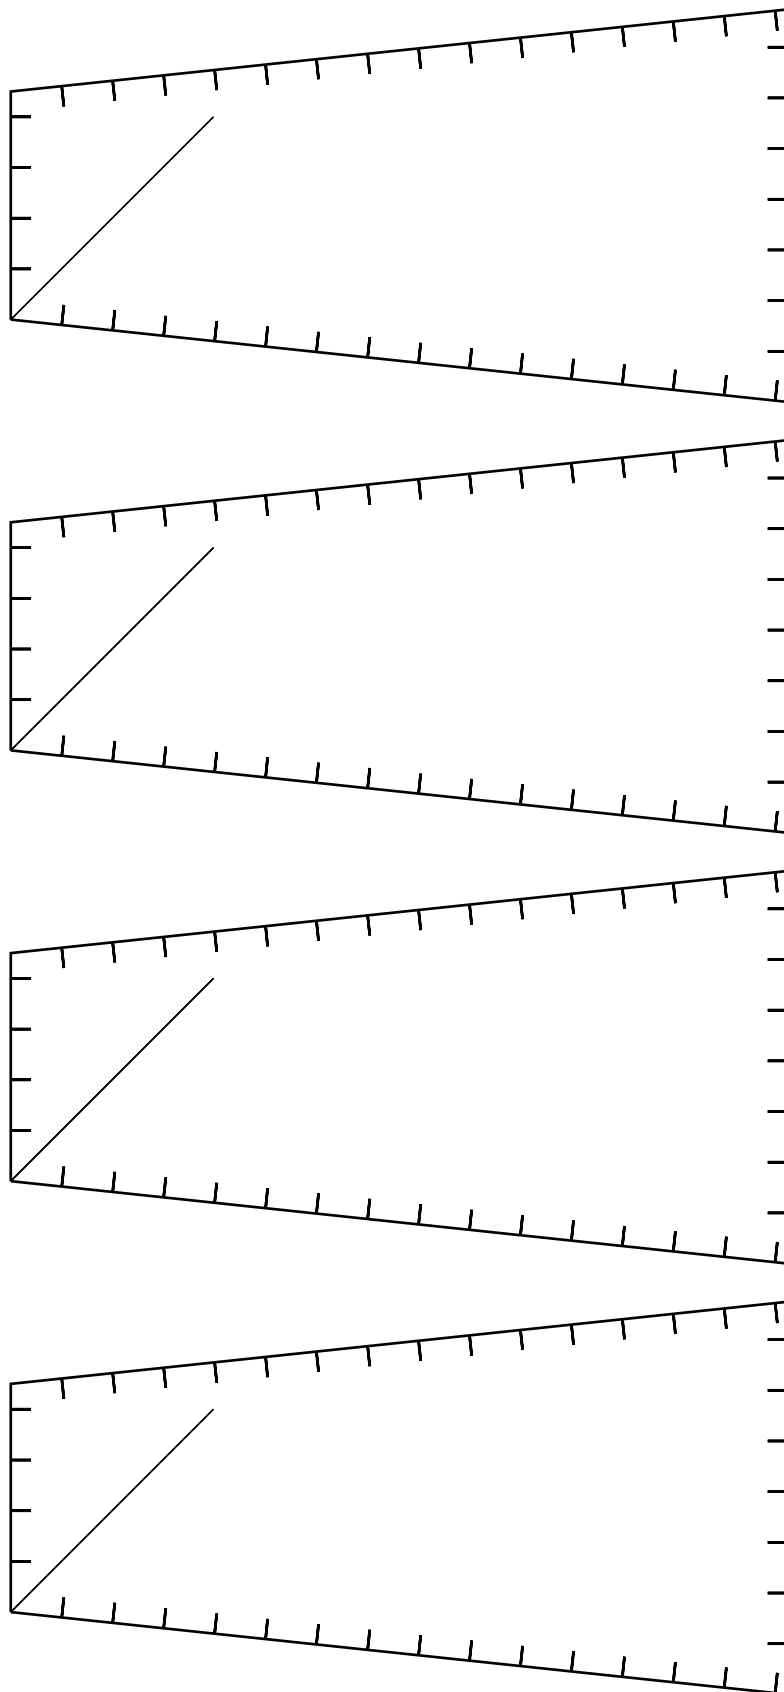

# Sector model of the spacetime of a radial ray in the exterior region of a black hole

With markings for two light signals

## Sektormodell für die Raumzeit eines radialen Strahls im Außenraum eines Schwarzen Lochs

Mit Startstrichen für zwei Lichtsignale

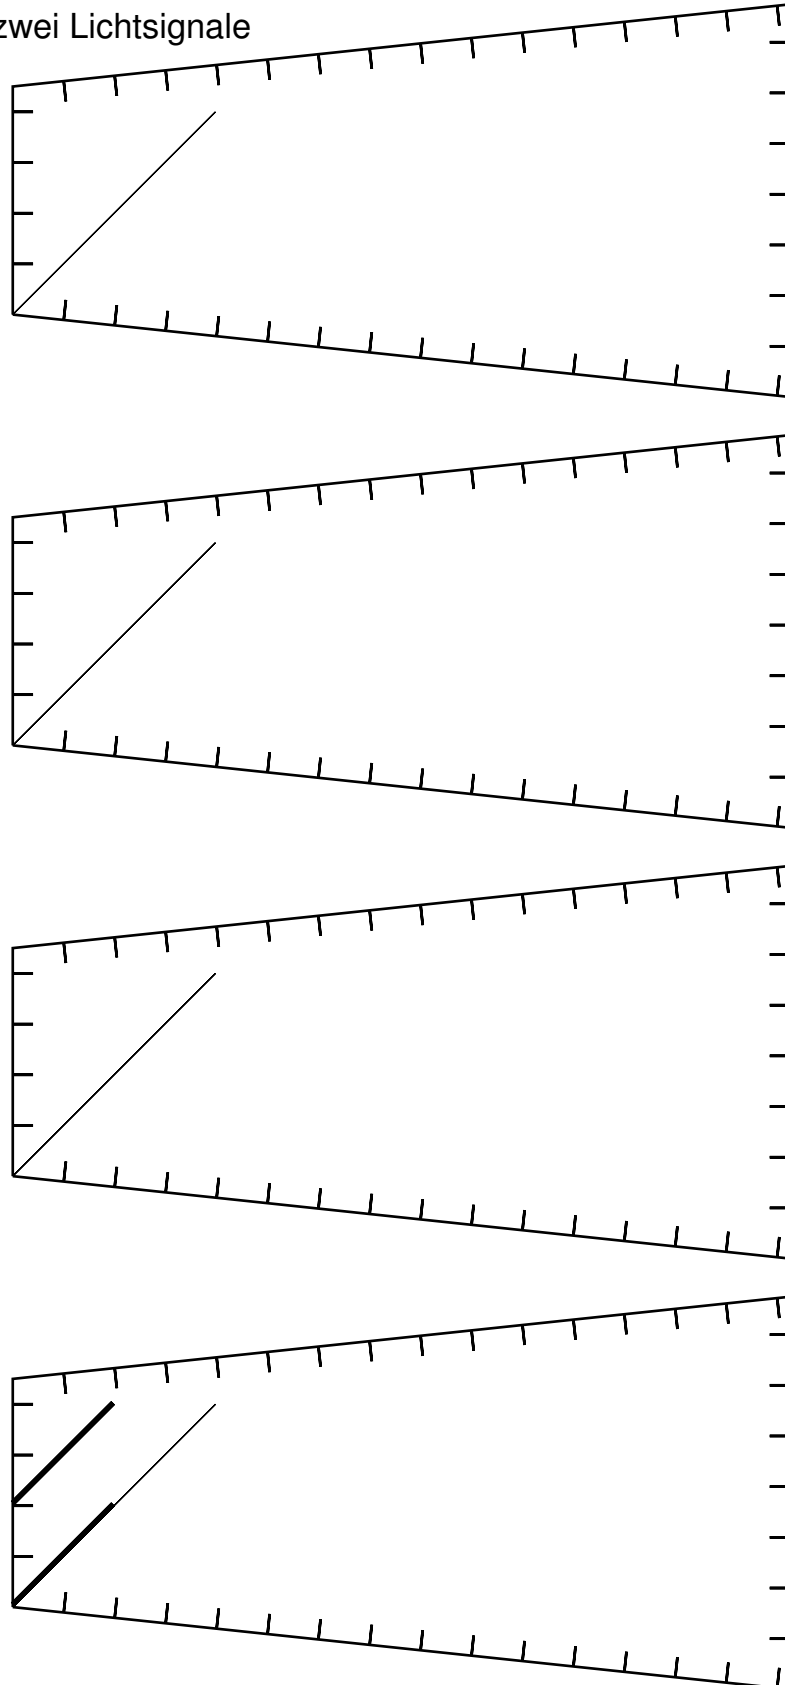

# Sector model of the spacetime of a radial ray in the exterior region of a black hole

With two light signals

## Sektormodell für die Raumzeit eines radialen Strahls im Außenraum eines Schwarzen Lochs

Mit zwei Lichtsignalen

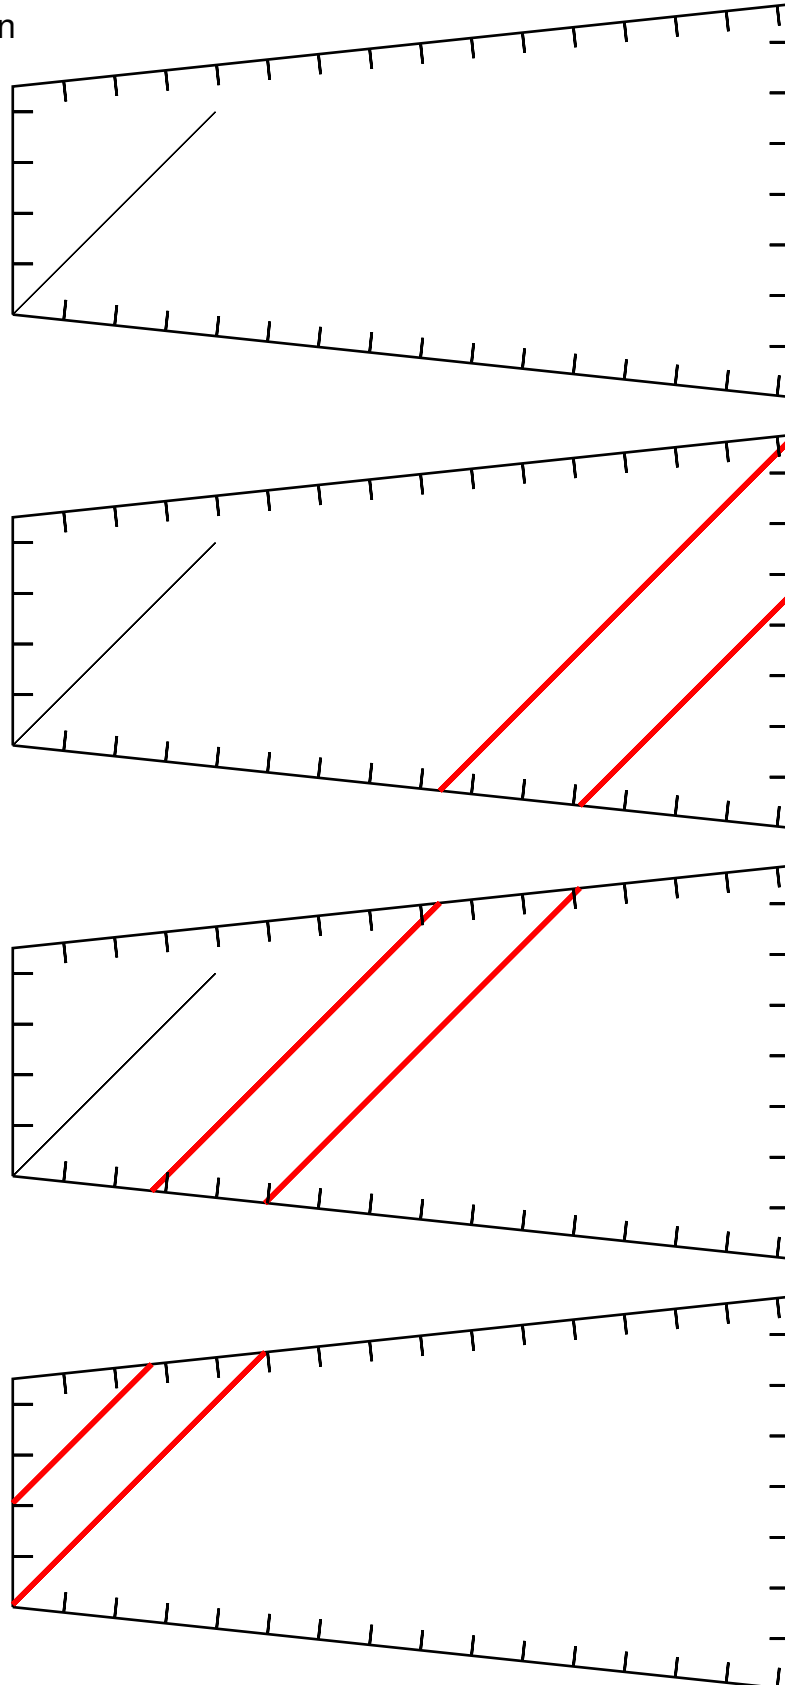

Sector model of the spacetime of a radial ray in the exterior region of a black hole

Sektormodell für die Raumzeit eines radialen Strahls im Außenraum eines Schwarzen Lochs

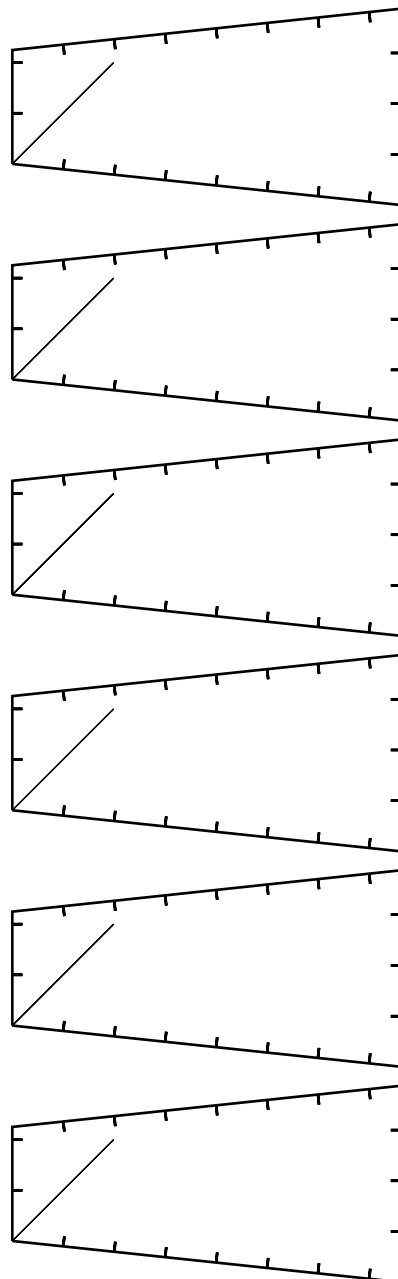

# Sector model of the spacetime of a radial ray in the exterior region of a black hole

With markings for two light signals

## Sektormodell für die Raumzeit eines radialen Strahls im Außenraum eines Schwarzen Lochs

Mit Startstrichen für zwei Lichtsignale

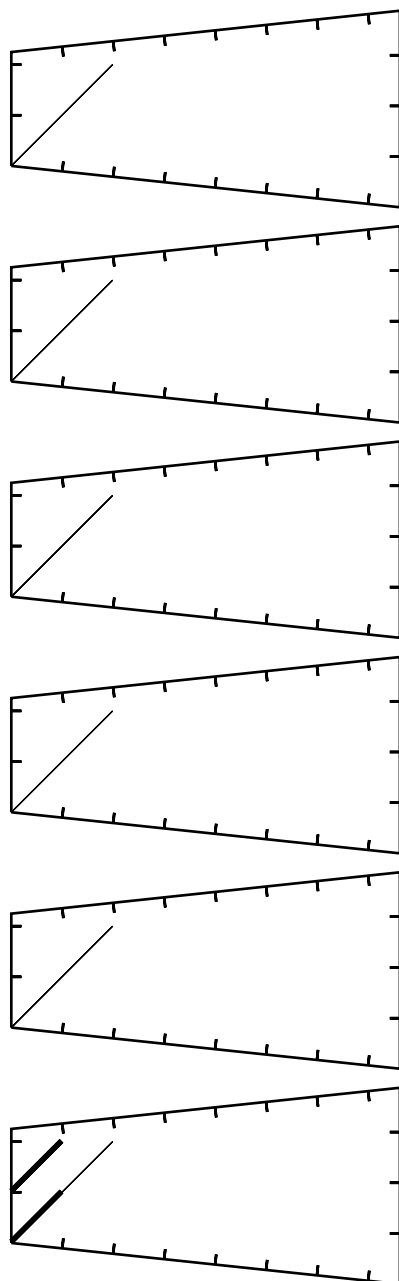

# Sector model of the spacetime of a radial ray in the exterior region of a black hole

With two light signals

## Sektormodell für die Raumzeit eines radialen Strahls im Außenraum eines Schwarzen Lochs

Mit zwei Lichtsignalen

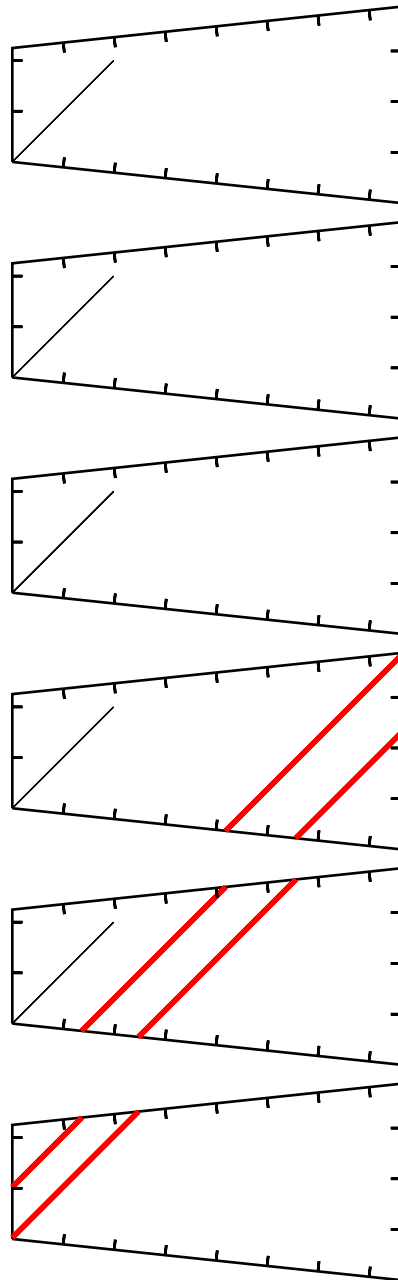



# Sector model of the spacetime of a radial ray in the exterior region of a black hole

With marking for path of particle thrown upwards

## Sektormodell für die Raumzeit eines radialen Strahls im Außenraum eines Schwarzen Lochs

Mit Startstrich für senkrechten Wurf nach oben

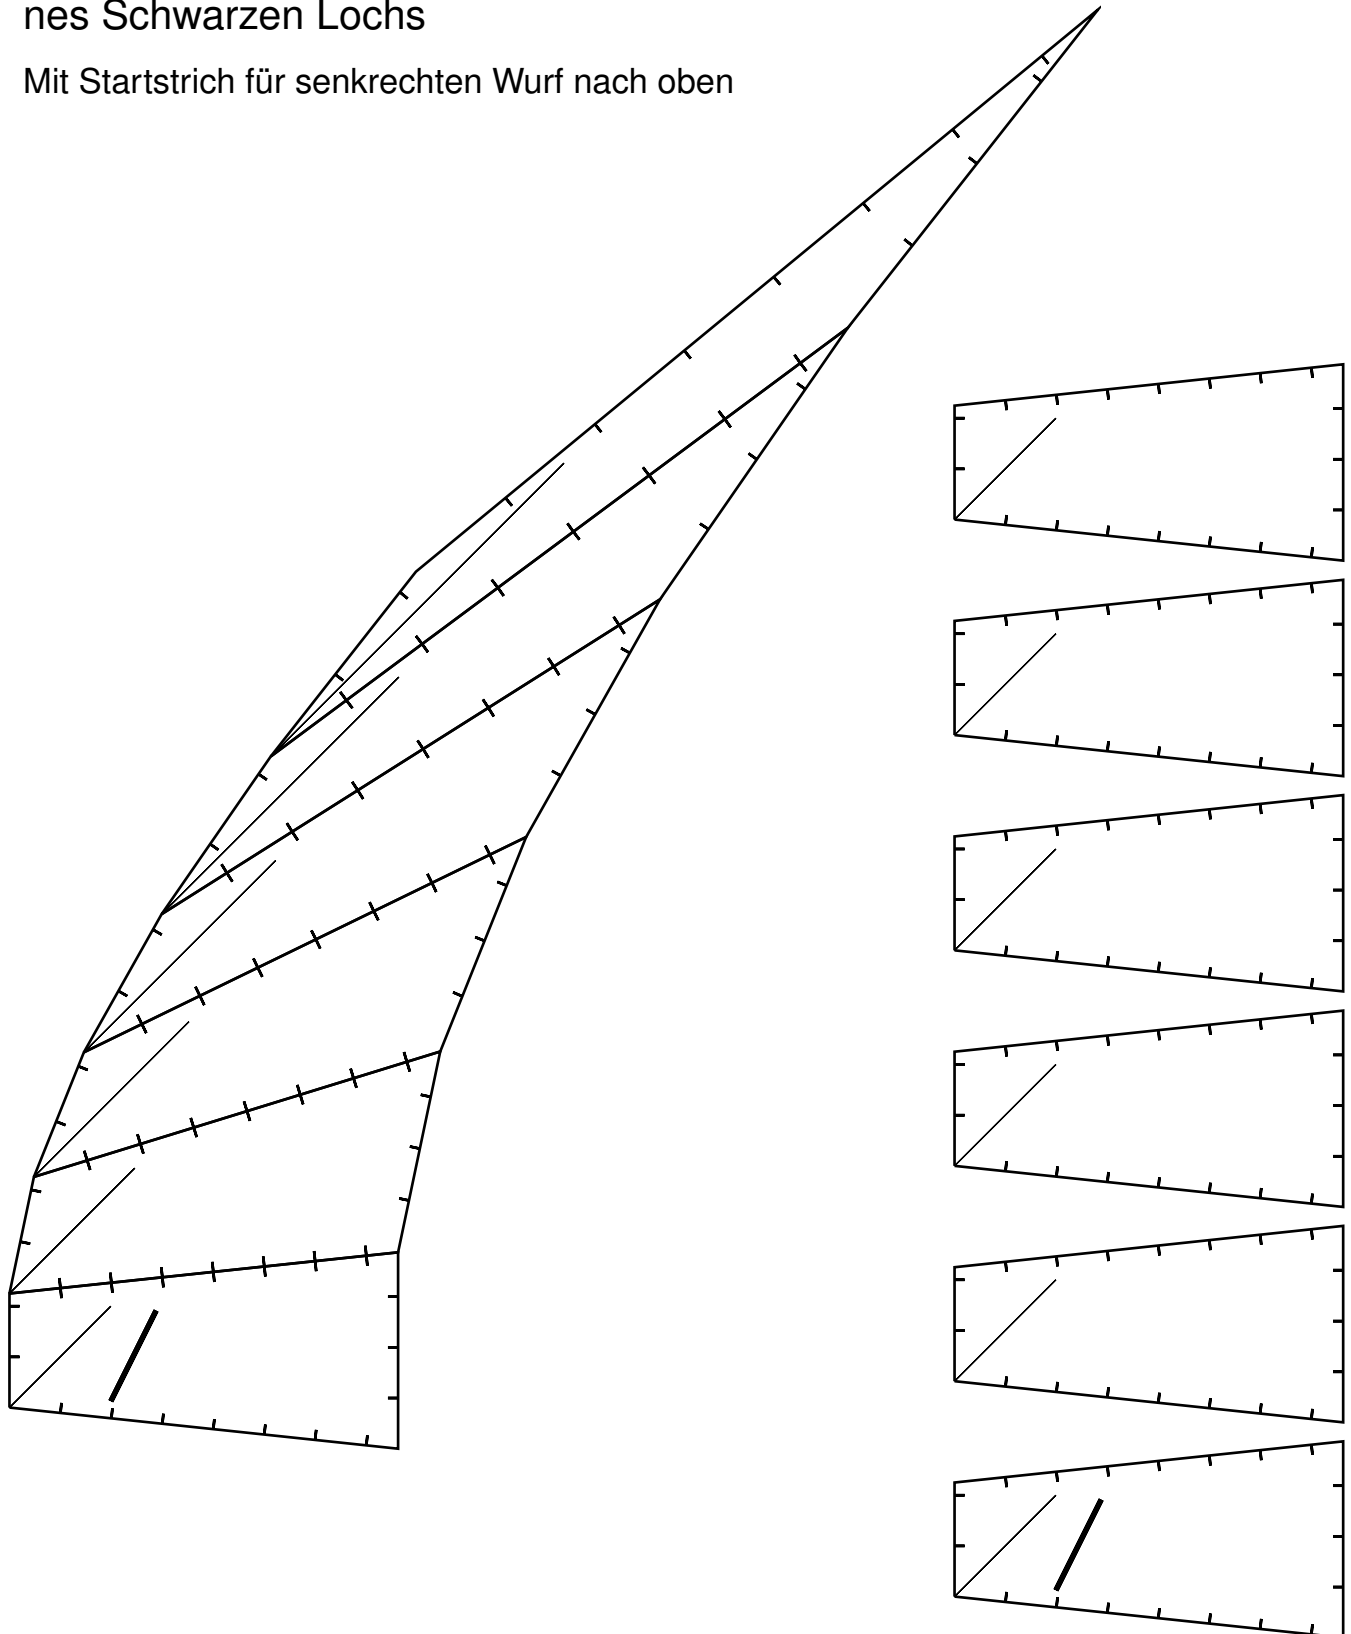

# Sector model of the spacetime of a radial ray in the exterior region of a black hole

With world line of a particle thrown upwards

## Sektormodell für die Raumzeit eines radialen Strahls im Außenraum eines Schwarzen Lochs

Mit Weltlinie eines nach oben geworfenen Teilchens

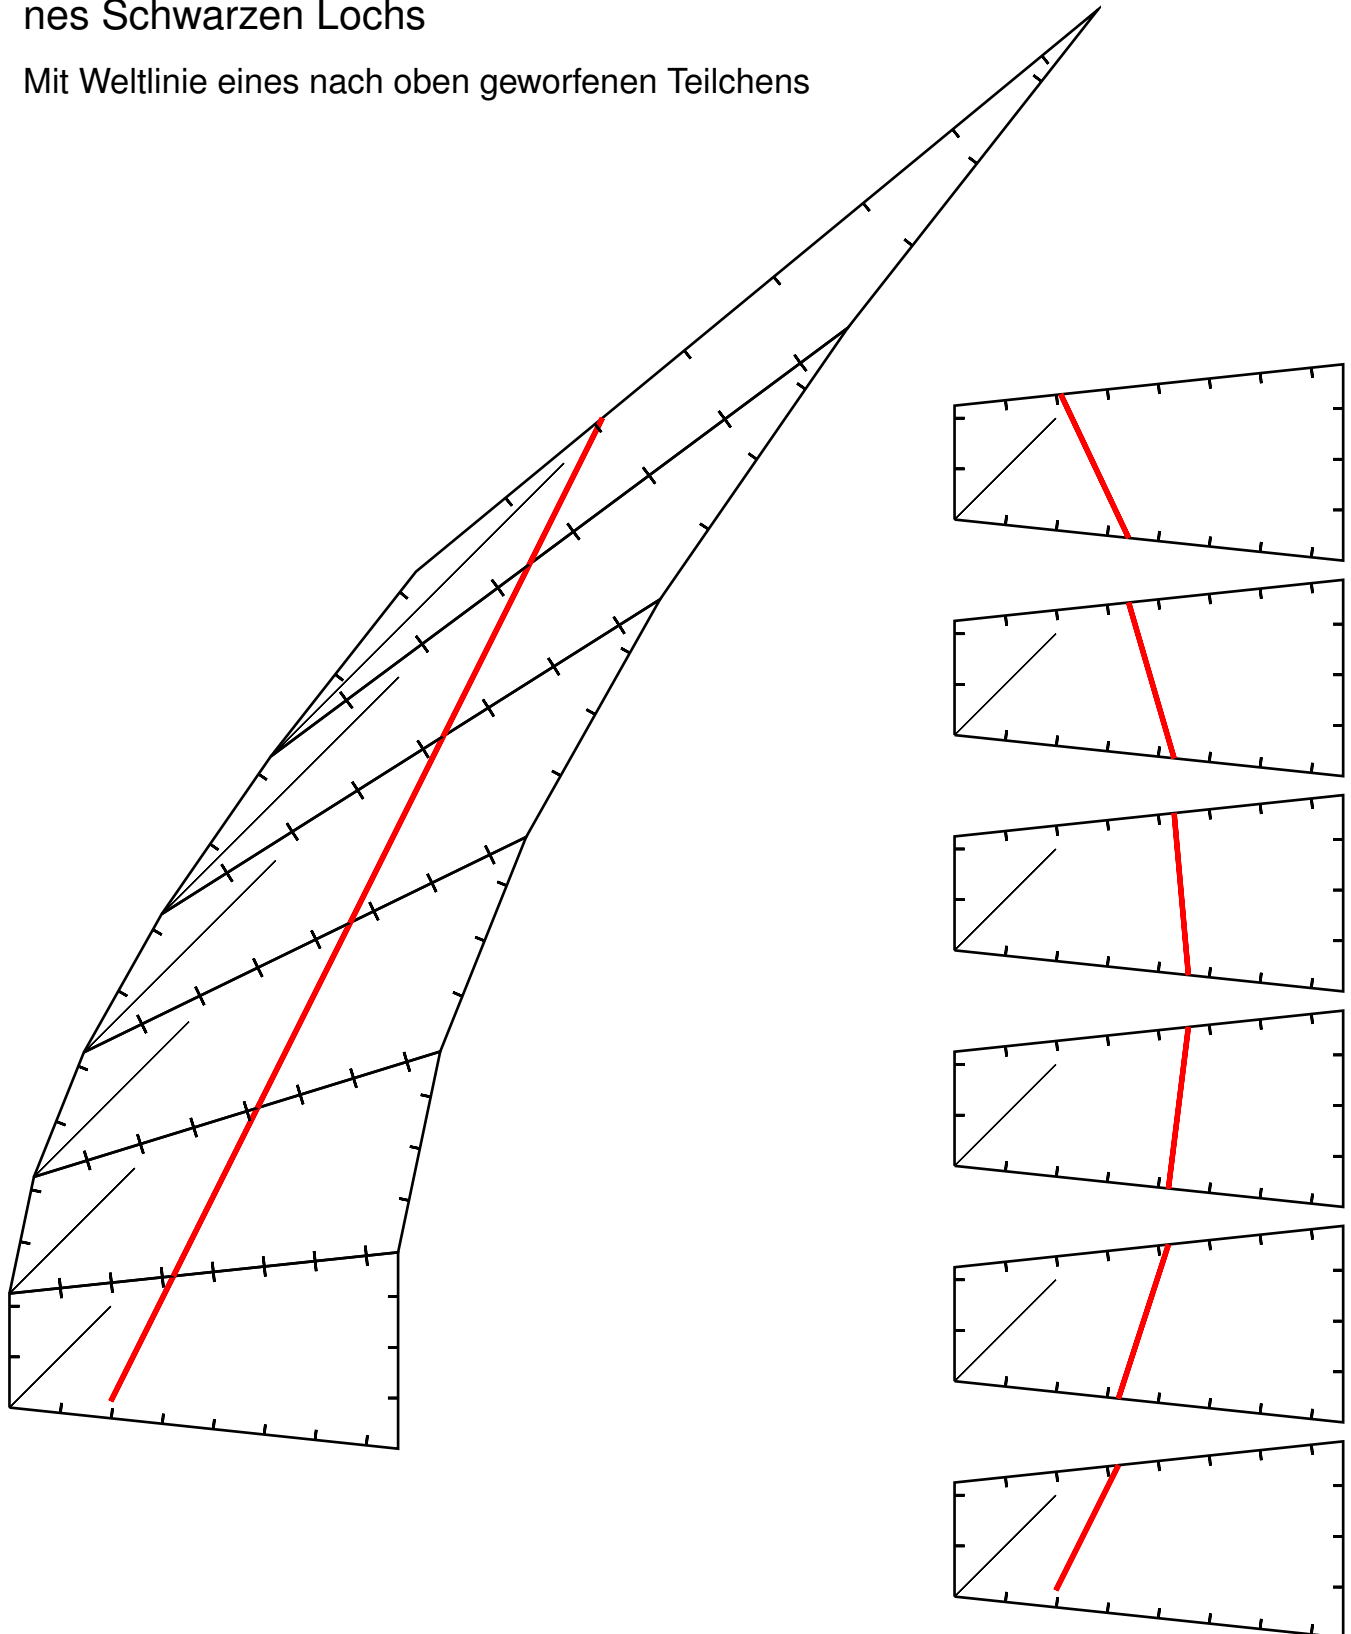

# Sector model of the spacetime of a radial ray in the exterior region of a black hole

With transfer sector

## Sektormodell für die Raumzeit eines radialen Strahls im Außenraum eines Schwarzen Lochs

Mit Transfersektor

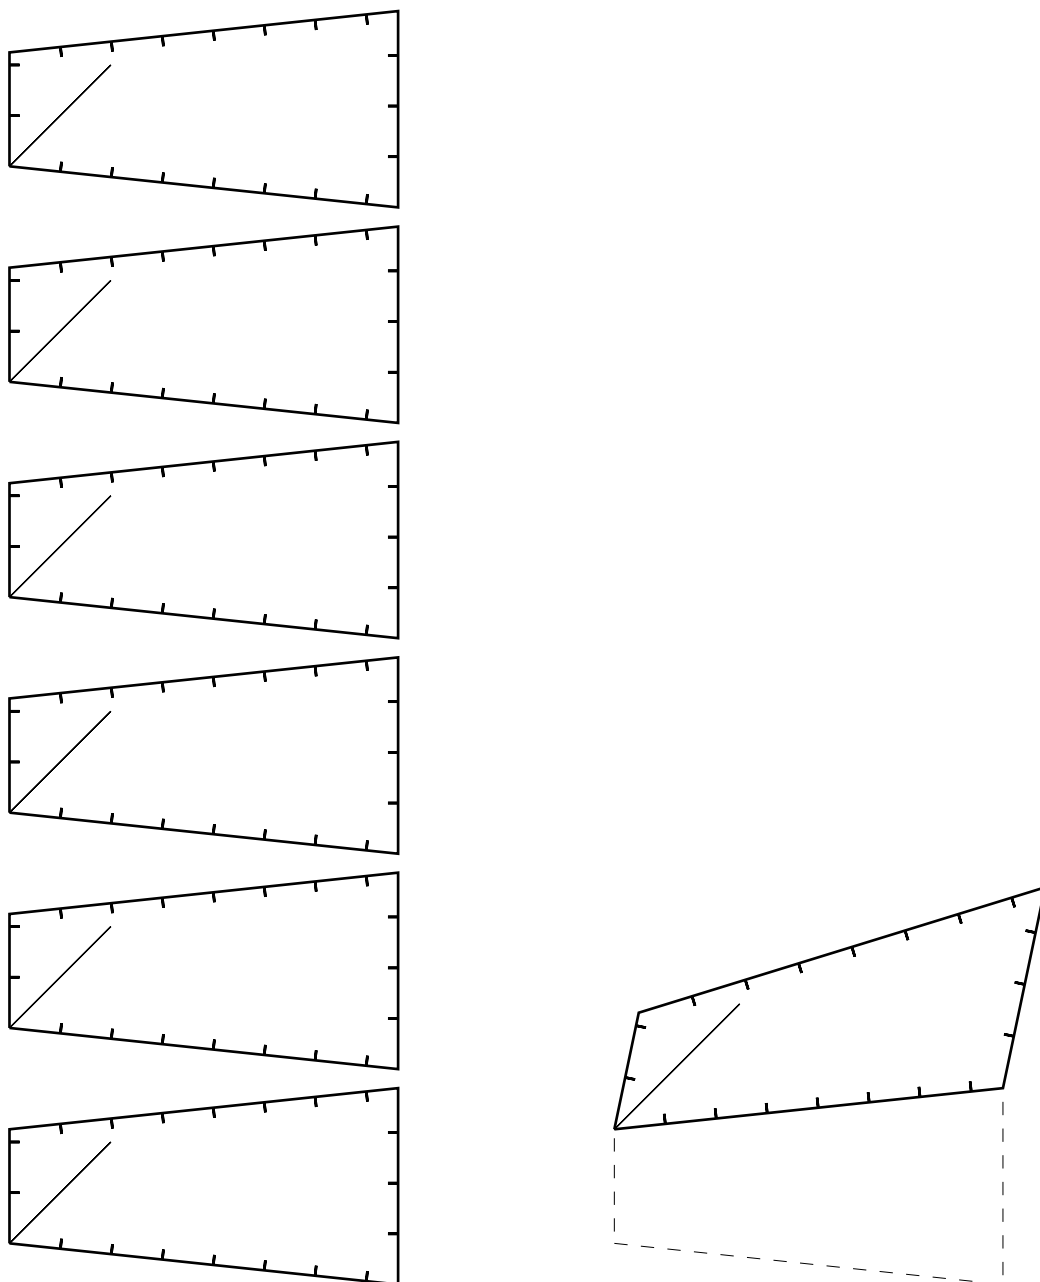

# Sector model of the spacetime of a radial ray in the exterior region of a black hole

With transfer sector and marking for path of particle thrown upwards

## Sektormodell für die Raumzeit eines radialen Strahls im Außenraum eines Schwarzen Lochs

Mit Transfersektor und Startstrich für senkrechten Wurf nach oben

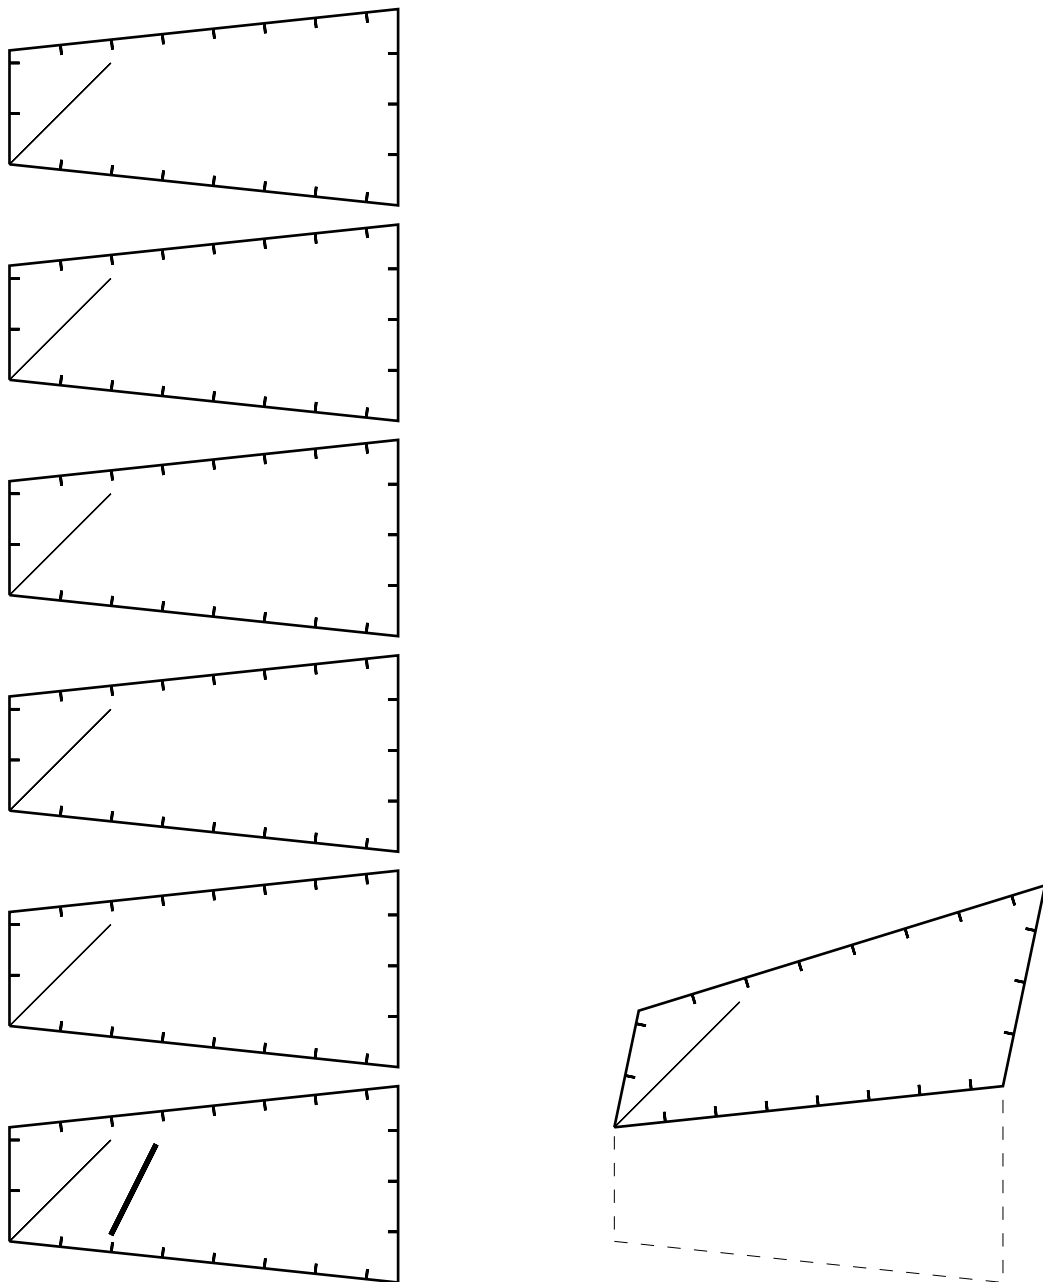

# Sector model of the spacetime of a radial ray in the exterior region of a black hole

With world line of a particle thrown upwards

## Sektormodell für die Raumzeit eines radialen Strahls im Außenraum eines Schwarzen Lochs

Mit Weltlinie eines nach oben geworfenen Teilchens

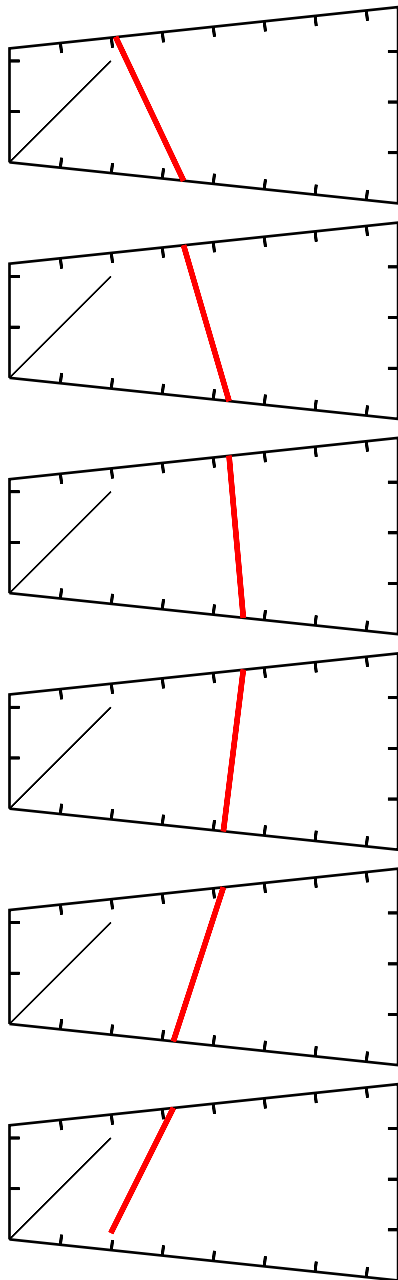

Sector model of the space-time of a radial ray in the exterior region of a black hole

Sektormodell für die Raumzeit eines radialen Strahls im Außenraum eines Schwarzen Lochs

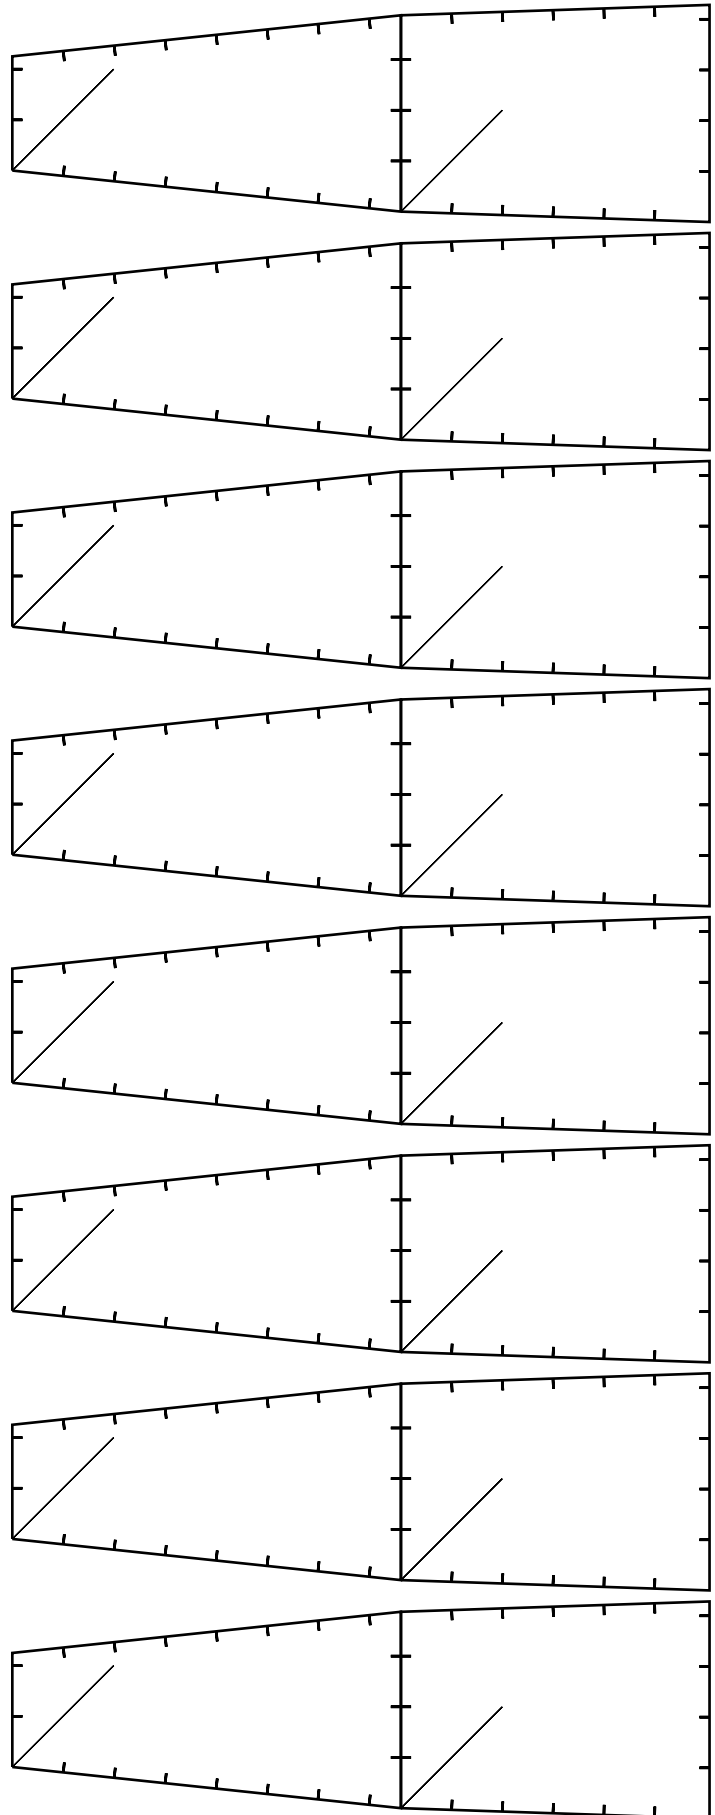

Sector model of the space-time of a radial ray in the exterior region of a black hole

With markings for two particles falling from rest

Sektormodell für die Raumzeit eines radialen Strahls im Außenraum eines Schwarzen Lochs

Mit Startstrichen für zwei aus der Ruhe fallende Teilchen

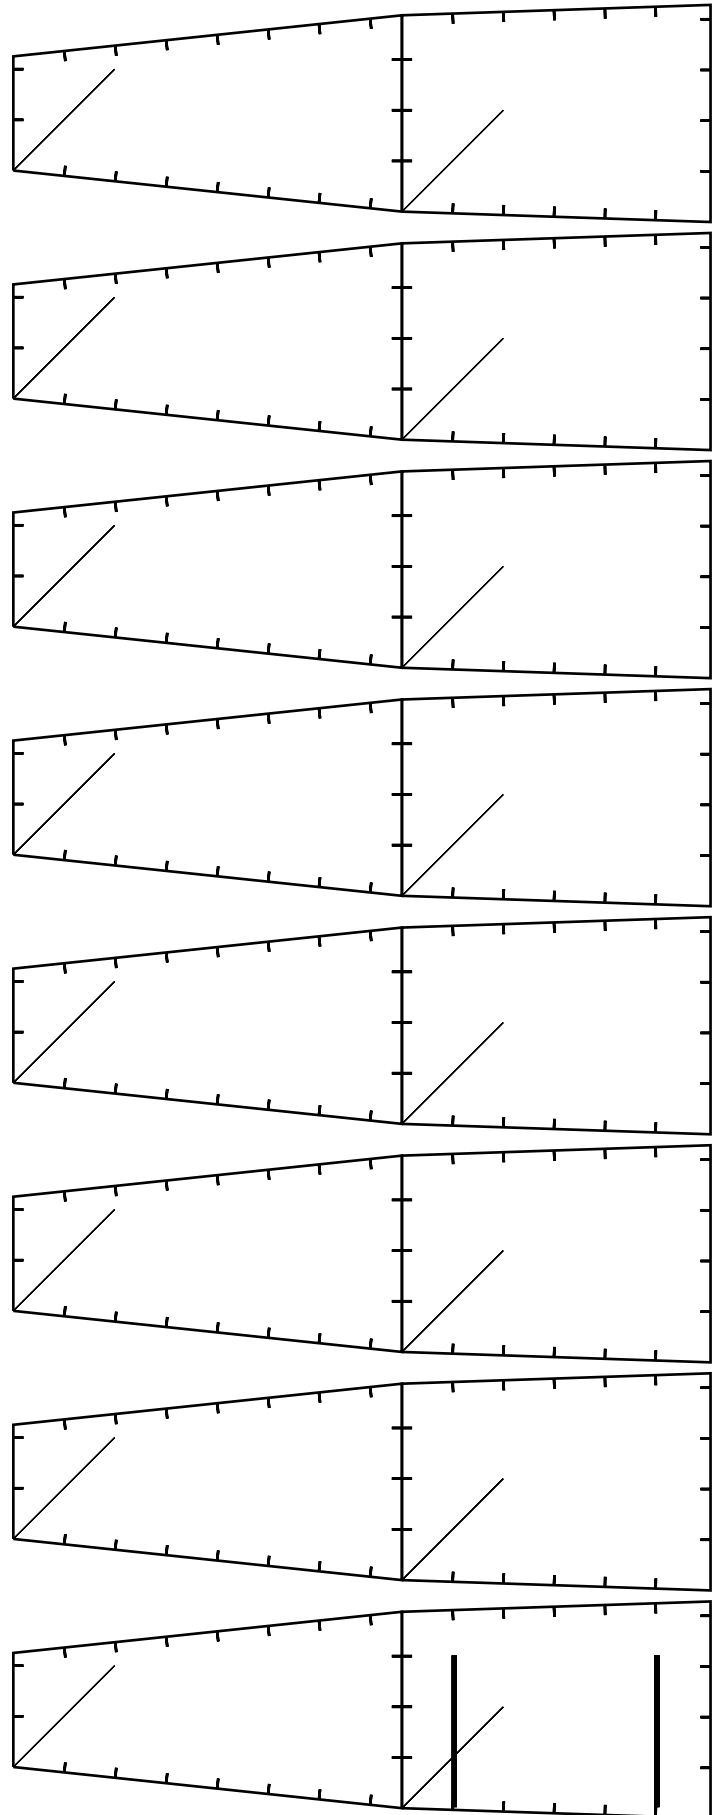

Sector model of the space-time of a radial ray in the exterior region of a black hole

With world lines for two particles falling from rest

Sektormodell für die Raumzeit eines radialen Strahls im Außenraum eines Schwarzen Lochs

Mit Weltlinien für zwei aus der Ruhe fallende Teilchen

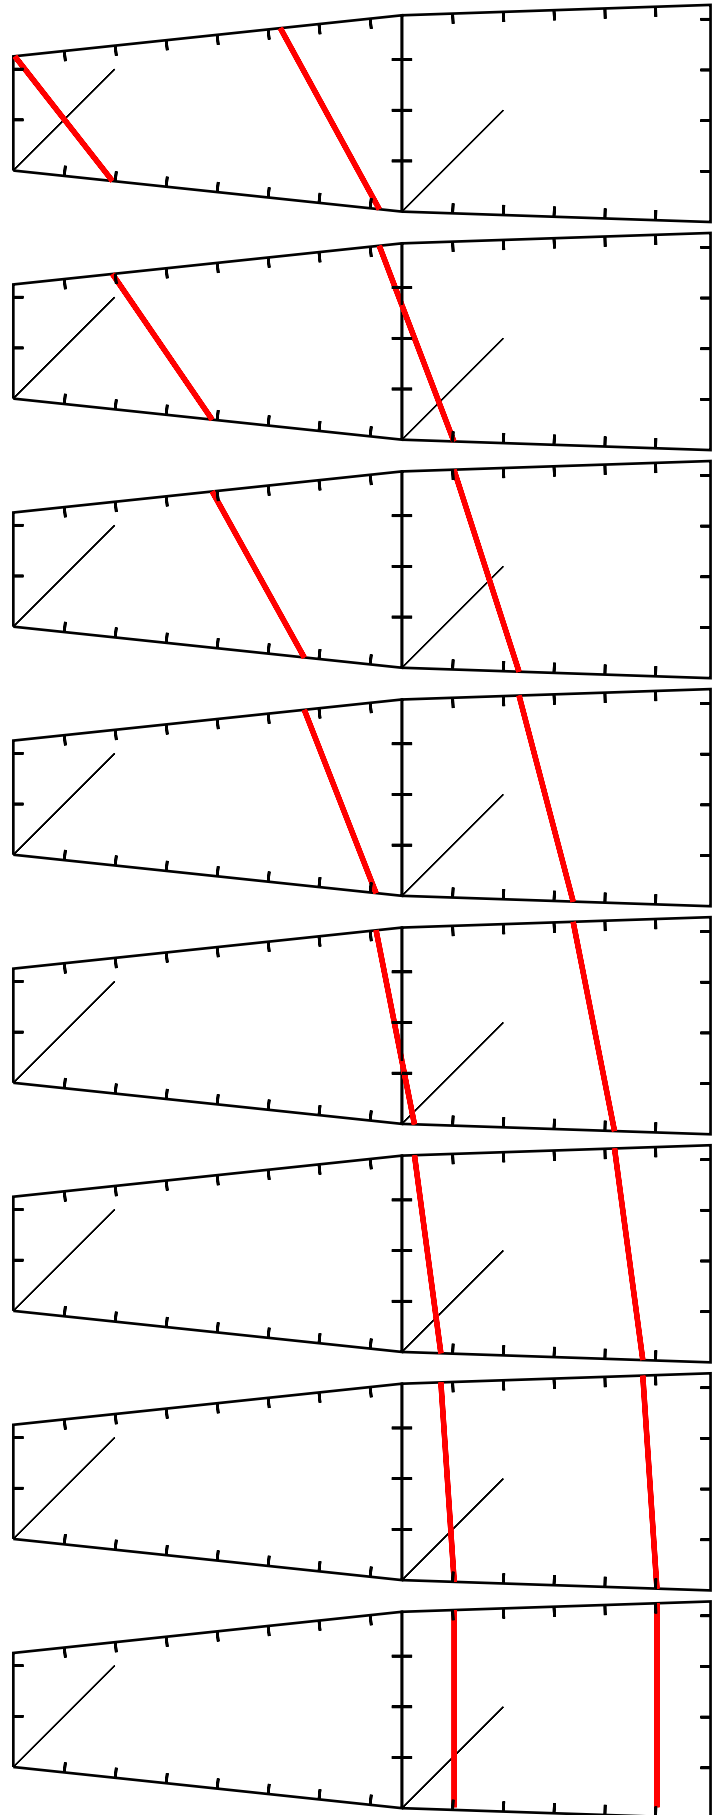



# Sector model of the spacetime of a radial ray in the exterior region of a black hole

Transfer sectors, transfer double sectors

## Sektormodell für die Raumzeit eines radialen Strahls im Außenraum eines Schwarzen Lochs

Transfersektoren, Transfer-Doppelsektoren

Transfer sector left column  
Transfersektor linke Spalte

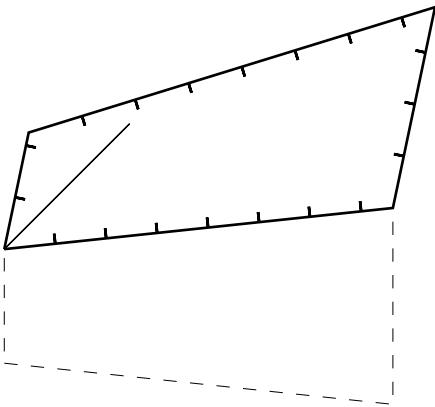

Transfer sector right column  
Transfersektor rechte Spalte

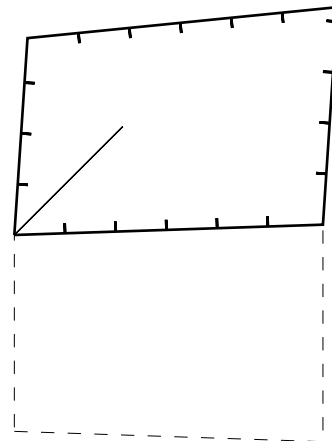

Transfer double sector left column  
Transfer-Doppelsektor linke Spalte

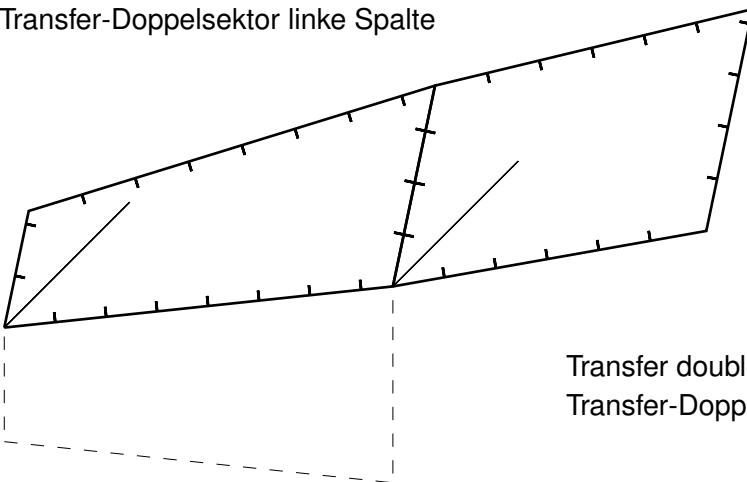

Transfer double sector right column  
Transfer-Doppelsektor rechte Spalte

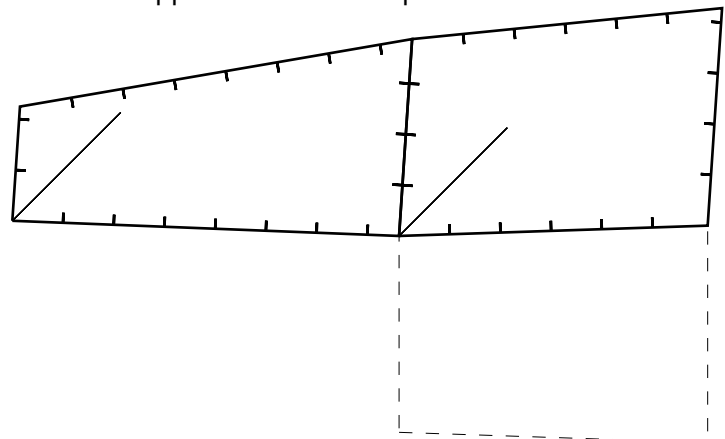

Supplement: Supplementary file 1 [file worksheets3.pdf]
